# Supplementary material for: Multimodal Label Relevance Ranking via Reinforcement Learning
Source: arXiv:2407.13221 source file (2024-07-18)
Supplement: Supplementary file 1 [file qualitative_supp.pdf]

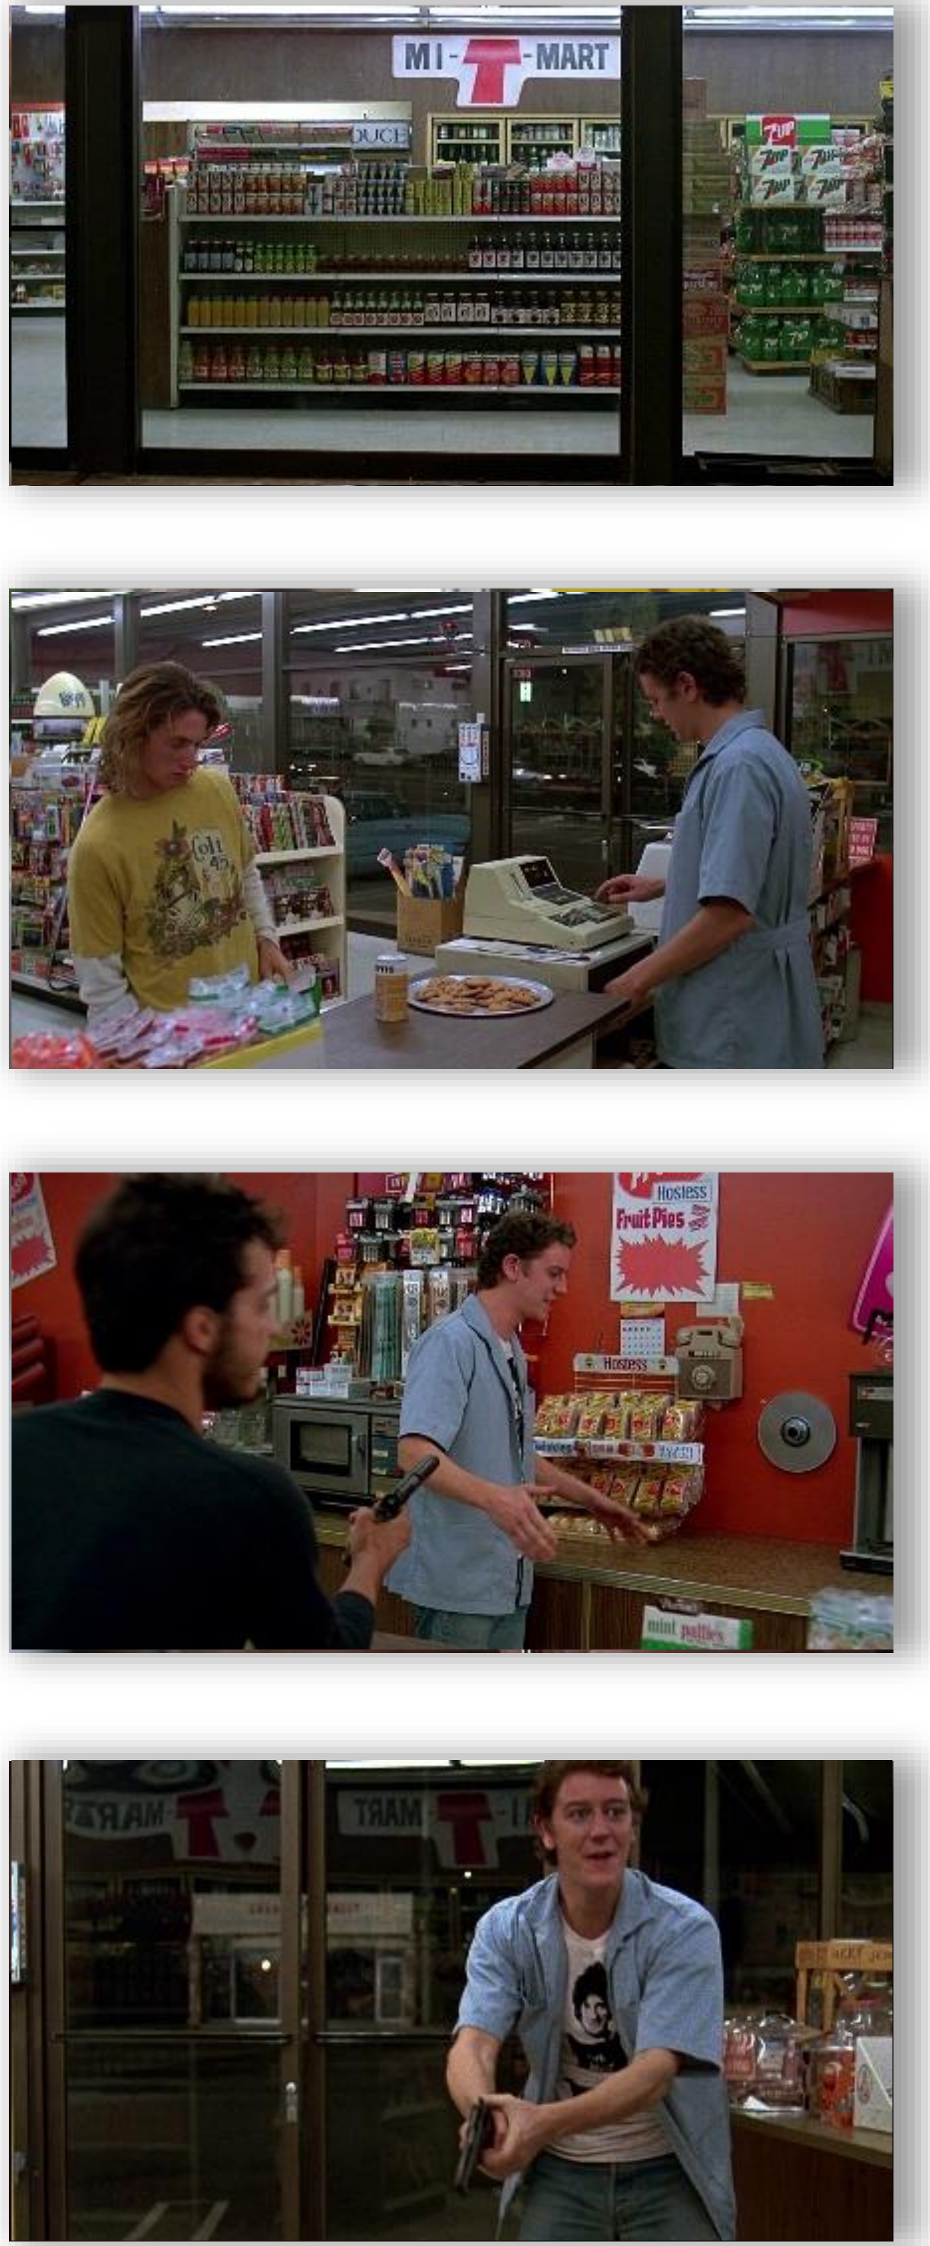


Meanwhile, Brad is working at his new job, the bottom rung on the high school scale of after-school employment: a convenience store called Mi-T-Mart. Spicoli walks in and tries to make a purchase while fumbling with pocket change. He then asks to use the bathroom. A robber pulls up, walks in the door, sprays the security camera, pulls out a pistol and tells Brad to give him all the money in the safe. Brad gets very nervous, and cannot open the safe, but then his fear turn into anger as he mouths off to the armed robber, wishing that he would just die, as Brad sees this as just one more rotten episode in his disintegrating life. Spicoli walks out of the bathroom and inadvertently distracts the thief just long enough for a furious Brad to throw a pot of hot coffee in the robber's face, jump over the counter, take his gun away and capture the would-be thief as the criminal's getaway car peels out the parking lot, making Brad a local hero, at least in Spicoli's eyes.

| | | | | |
|---|---|---|---|---|
| High | robber | convenience store | local hero | criminal escapes |
| Medium | security camera | hot coffee | new job | cannot open safe |
| Low | thief distracted | gun taken away | getaway car | change |

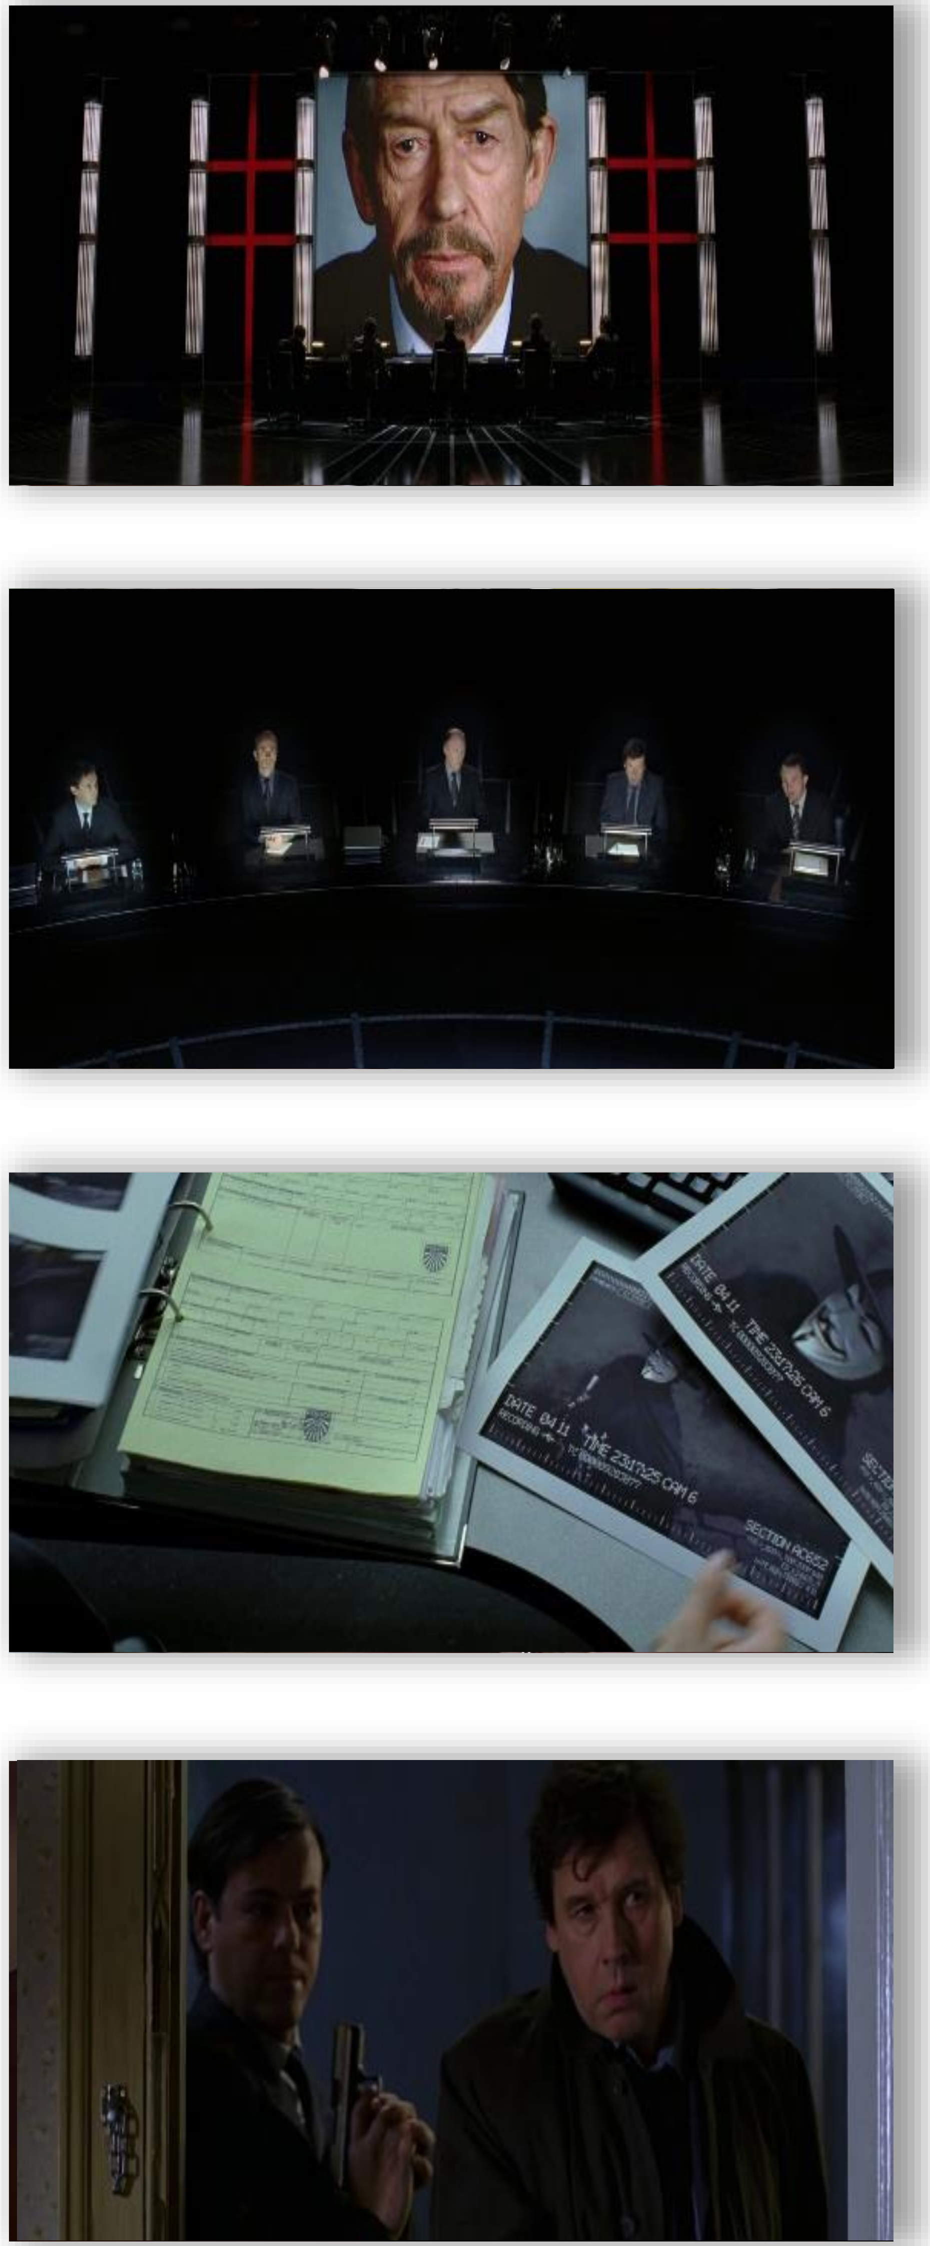

Following the explosion, a congregation of Norsefire's elite meets in a secret conference with Adam Sutler, his face projected on a large screen. Included are Inspector Eric Finch of the police, Roger Dascomb of television broadcasting, Brian Etheridge of the auditory surveillance system, Peter Creedy of the secret police, and Conrad Heyer of the CCTV. Effectively and respectively, they make up the nose, mouth, ears, fingers, and eyes of the government, with Sutler sitting at the brain. Sutler decrees that the destruction of The Old Bailey is to be announced as an impromptu demolition project to make way for a new building while an investigation ensues to find out who the man in the Fawkes mask is. While V's remains a mystery, Evey's identity is quickly discovered thanks to video surveillance and Sutler demands her capture and interrogation.

| | |
|---|---|
| High | secret conference \| elite \| mystery identity \| mask man |
| Medium | interrogation \| video surveillance \| demand arrest \| big screen |
| Low | television broadcaster \| new building \| government mouth |

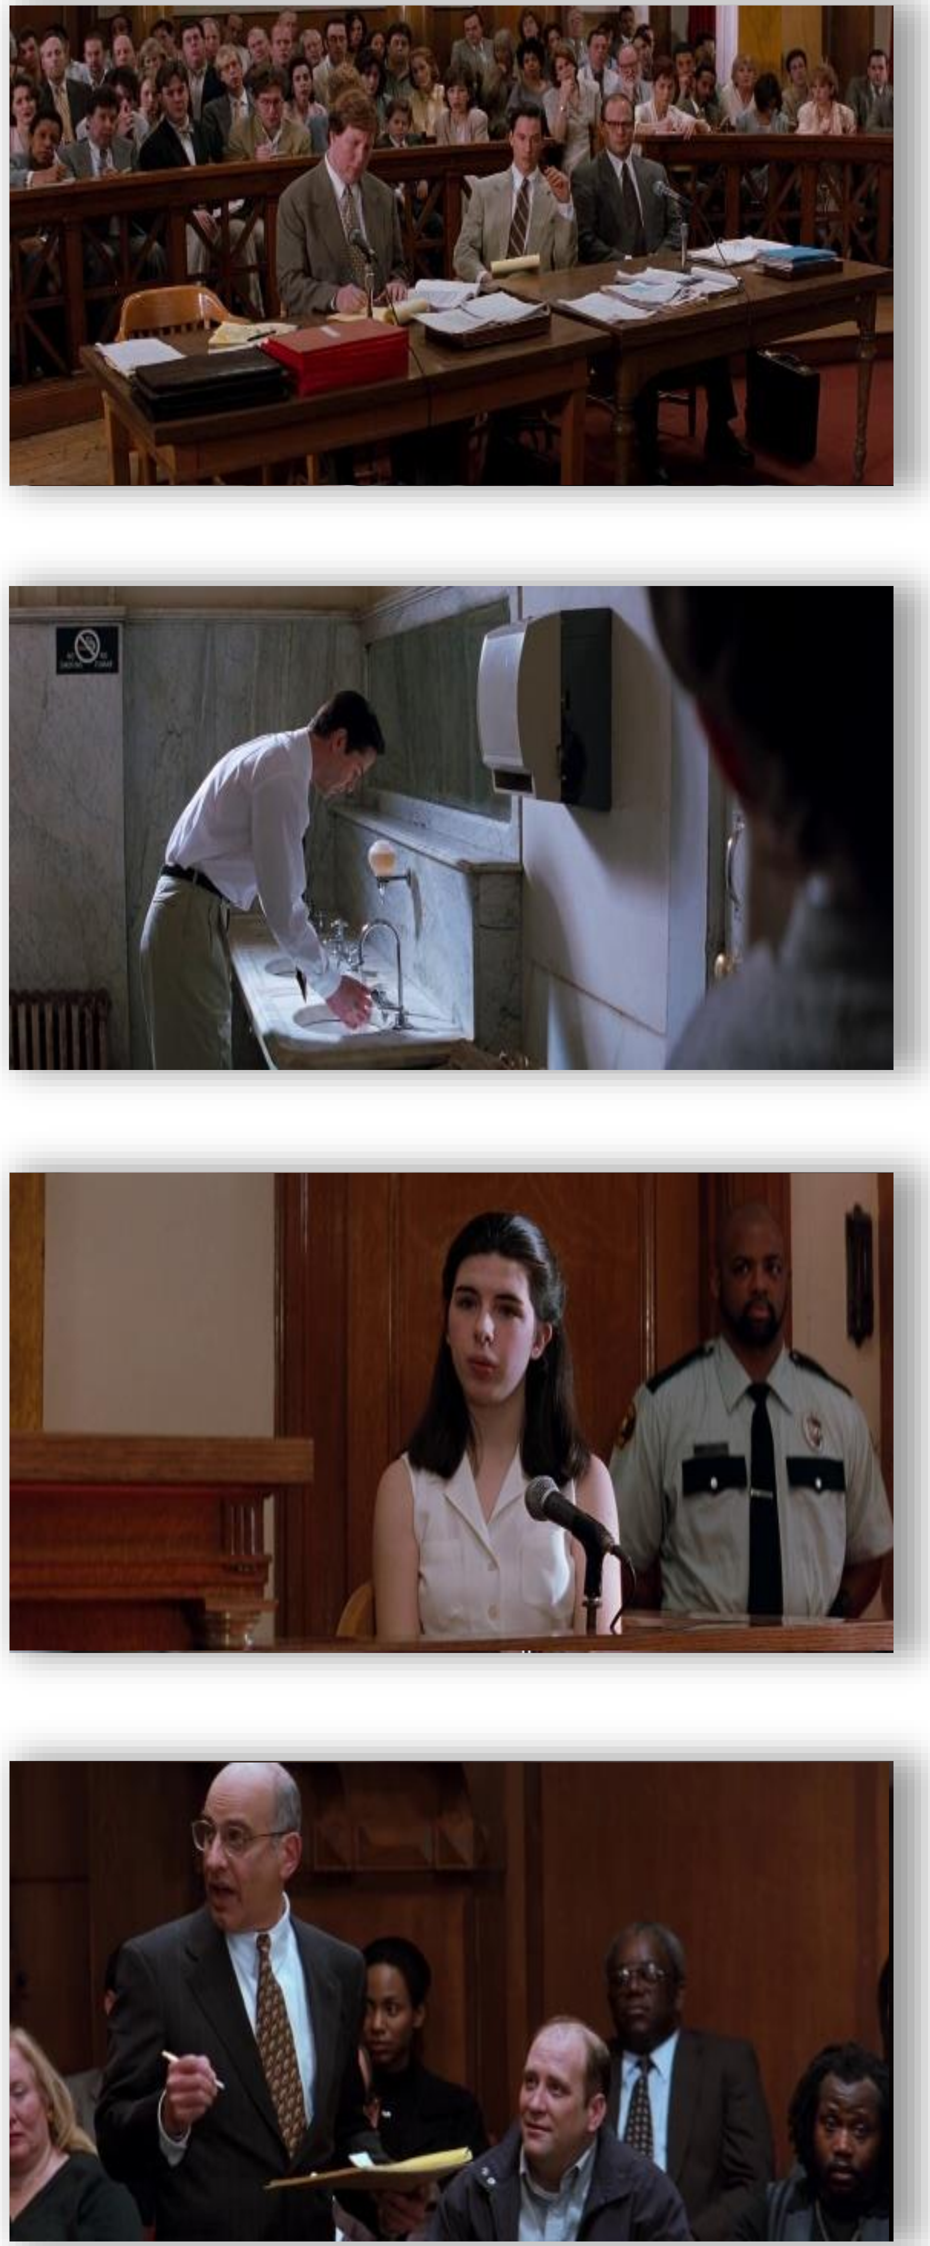

Kevin Lomax (Keanu Reeves) is a successful defense attorney in Gainesville, Florida. After successfully defending a high school teacher, Gettys, who is accused of molesting a young girl named Barbara (Heather Matarazzo). He is celebrating with his wife Mary Ann (Charlize Theron) when he is approached by a representative for a New York law firm, Leamon Heath (Ruben Santiago-Hudson). The Lomaxes go to New York, and Kevin proves his expertise while picking a jury. A sharply-dressed John Milton (Al Pacino) watches him from afar. The next day, Kevin receives word that Gettys has been acquitted. More so, the jury only deliberated for 38 minutes before bringing in the verdict.

| | | | | | | |
|---|---|---|---|---|---|---|
| success | > | crowd | \| | girl | > | architecture |
| lawyer | > | podium | \| | celebrate | > | police |
| girl | > | crowd | \| | represent | > | microphone |
| crowd | > | faucet | \| | success | > | clothing |
| court | > | suit | \| | crowd | > | architecture |

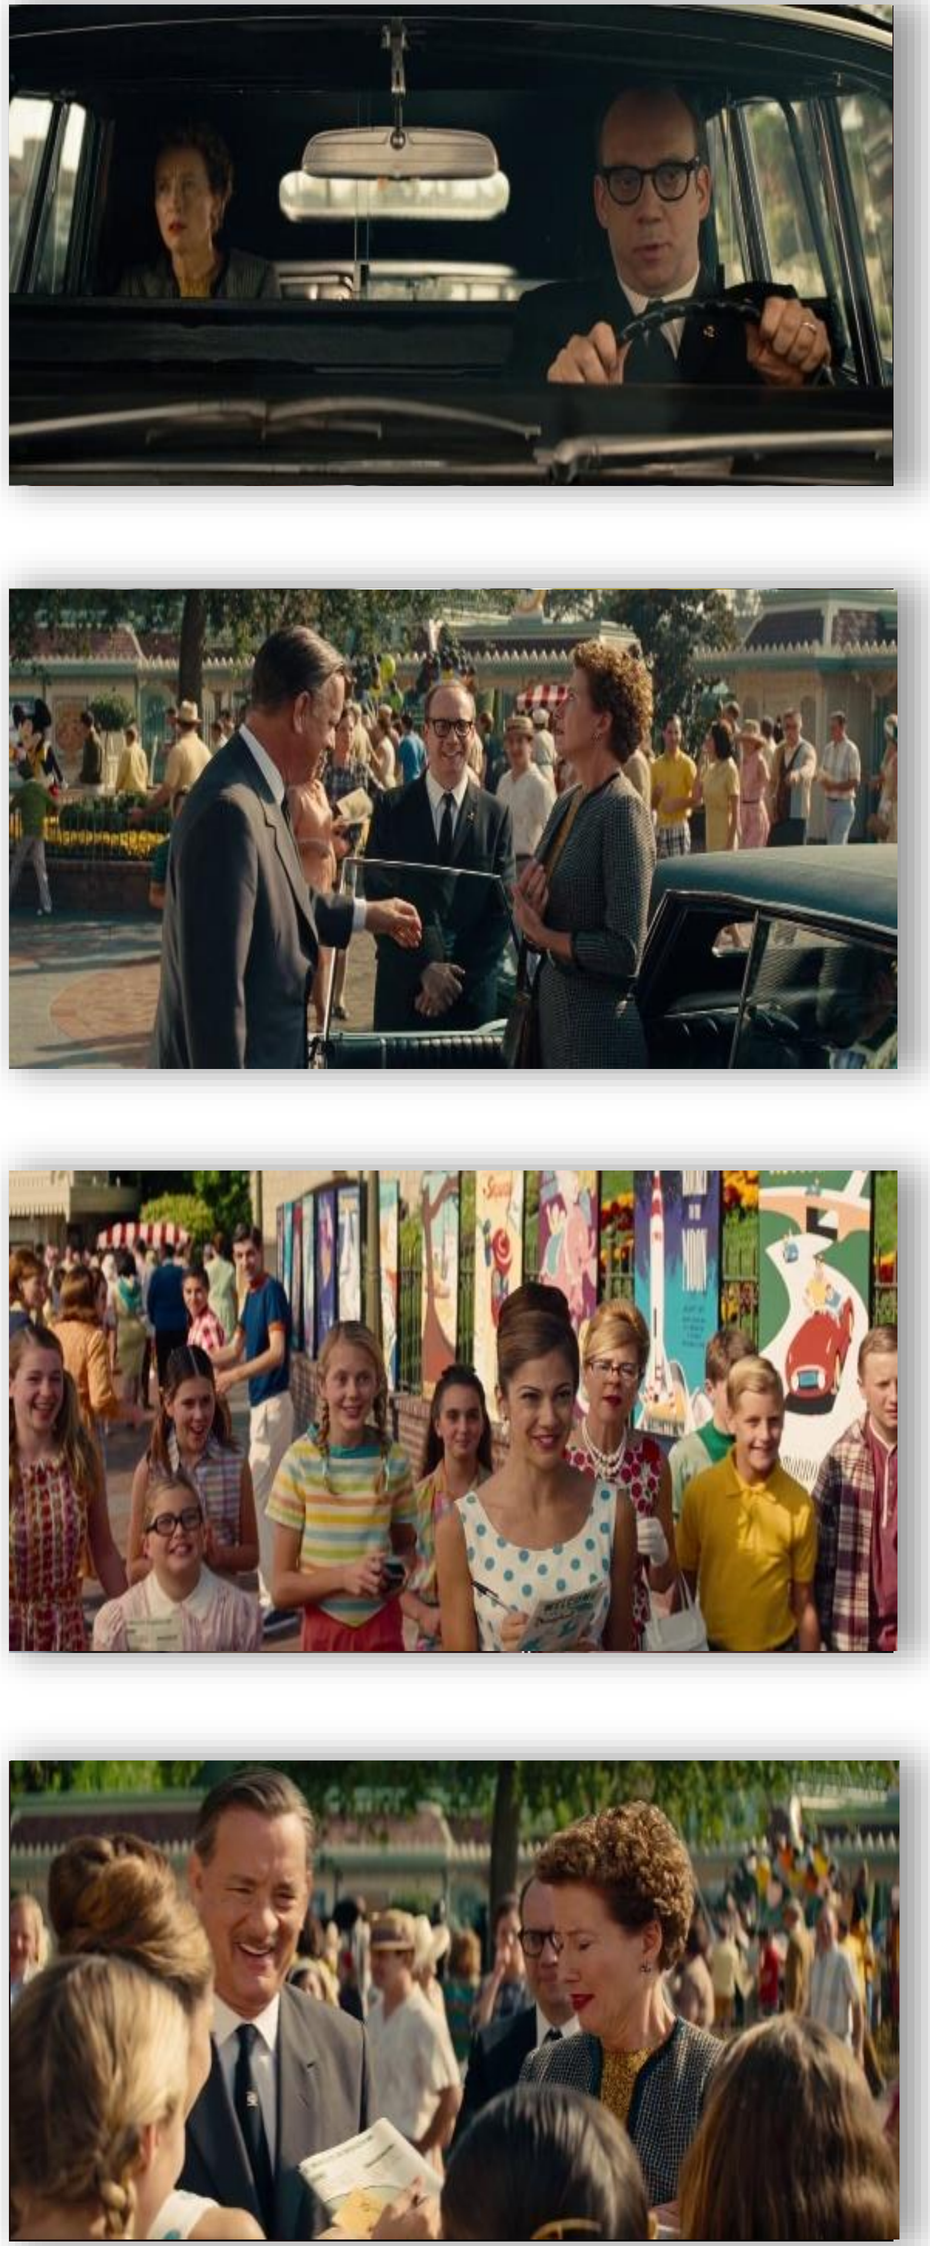

Ralph drives Pamela to Disneyland and they park on the property. Walt Disney greets them, exciting Ralph who has never met him in person; Pamela is not impressed though. The two walk through the park where young fans ask for Walt's autograph. Walt gives out pre-signed pictures, his method of dealing with attention when he goes to the park. Walt encourages the crowd to get Pamela's signature too and even though they happily offer her something to sign, she mockingly rejects them (possibly implying a case of inferiority complex).

| | | | | | | |
|---|---|---|---|---|---|---|
| amusement park | > | vehicle | \| | driver | > | seat |
| fans | > | exciting | \| | autograph | > | inferiority complex |
| crowd | > | black | \| | amusement park | > | laugh at |
| rejects requests | > | vehicle | \| | laugh at | > | wheel |
| inferiority complex | > | garden | \| | driver | > | garden |

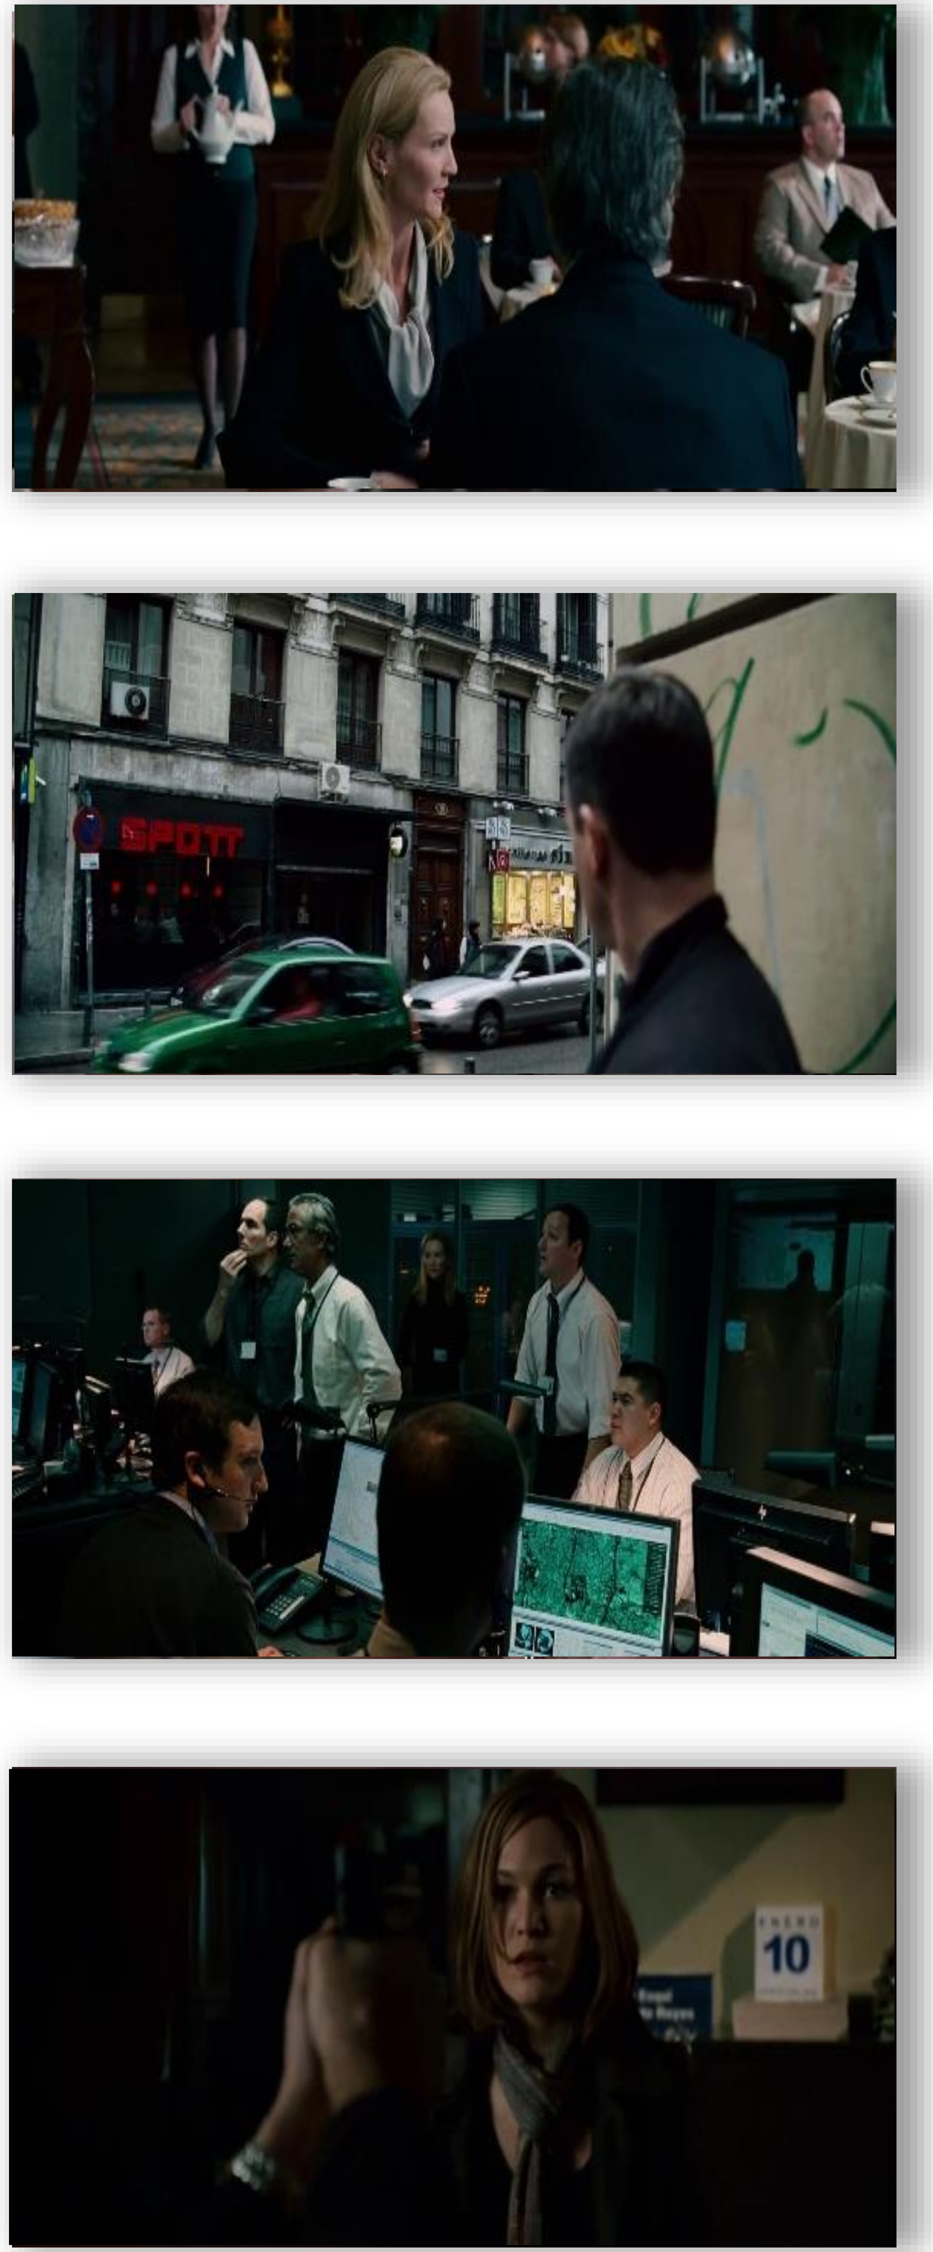

Pamela Landy, who had been assigned to hunt Bourne six weeks earlier, but was unsuccessful, is brought in to help Vosen. They search Ross's notes and find that Ross's source was Neal Daniels, the CIA station chief in Madrid, who was formerly involved in Treadstone and is involved in Blackbriar as well. Bourne makes his way to Daniels' Madrid office, but finds it empty. After Bourne incapacitates a CIA team sent by Vosen and Landy, Nicky Parsons, a former Treadstone support technician arrives. She decides to help Bourne and tells him that Daniels has fled to Tangier.

| | | | | | | | |
|---|---|---|---|---|---|---|---|
| High | hunt | Treadstone | Blackbriar | technician | | | |
| Medium | notes | station chief | office | table | crowd | city street | |
| Low | black | suit | tie | control | clean | dark | architecture |

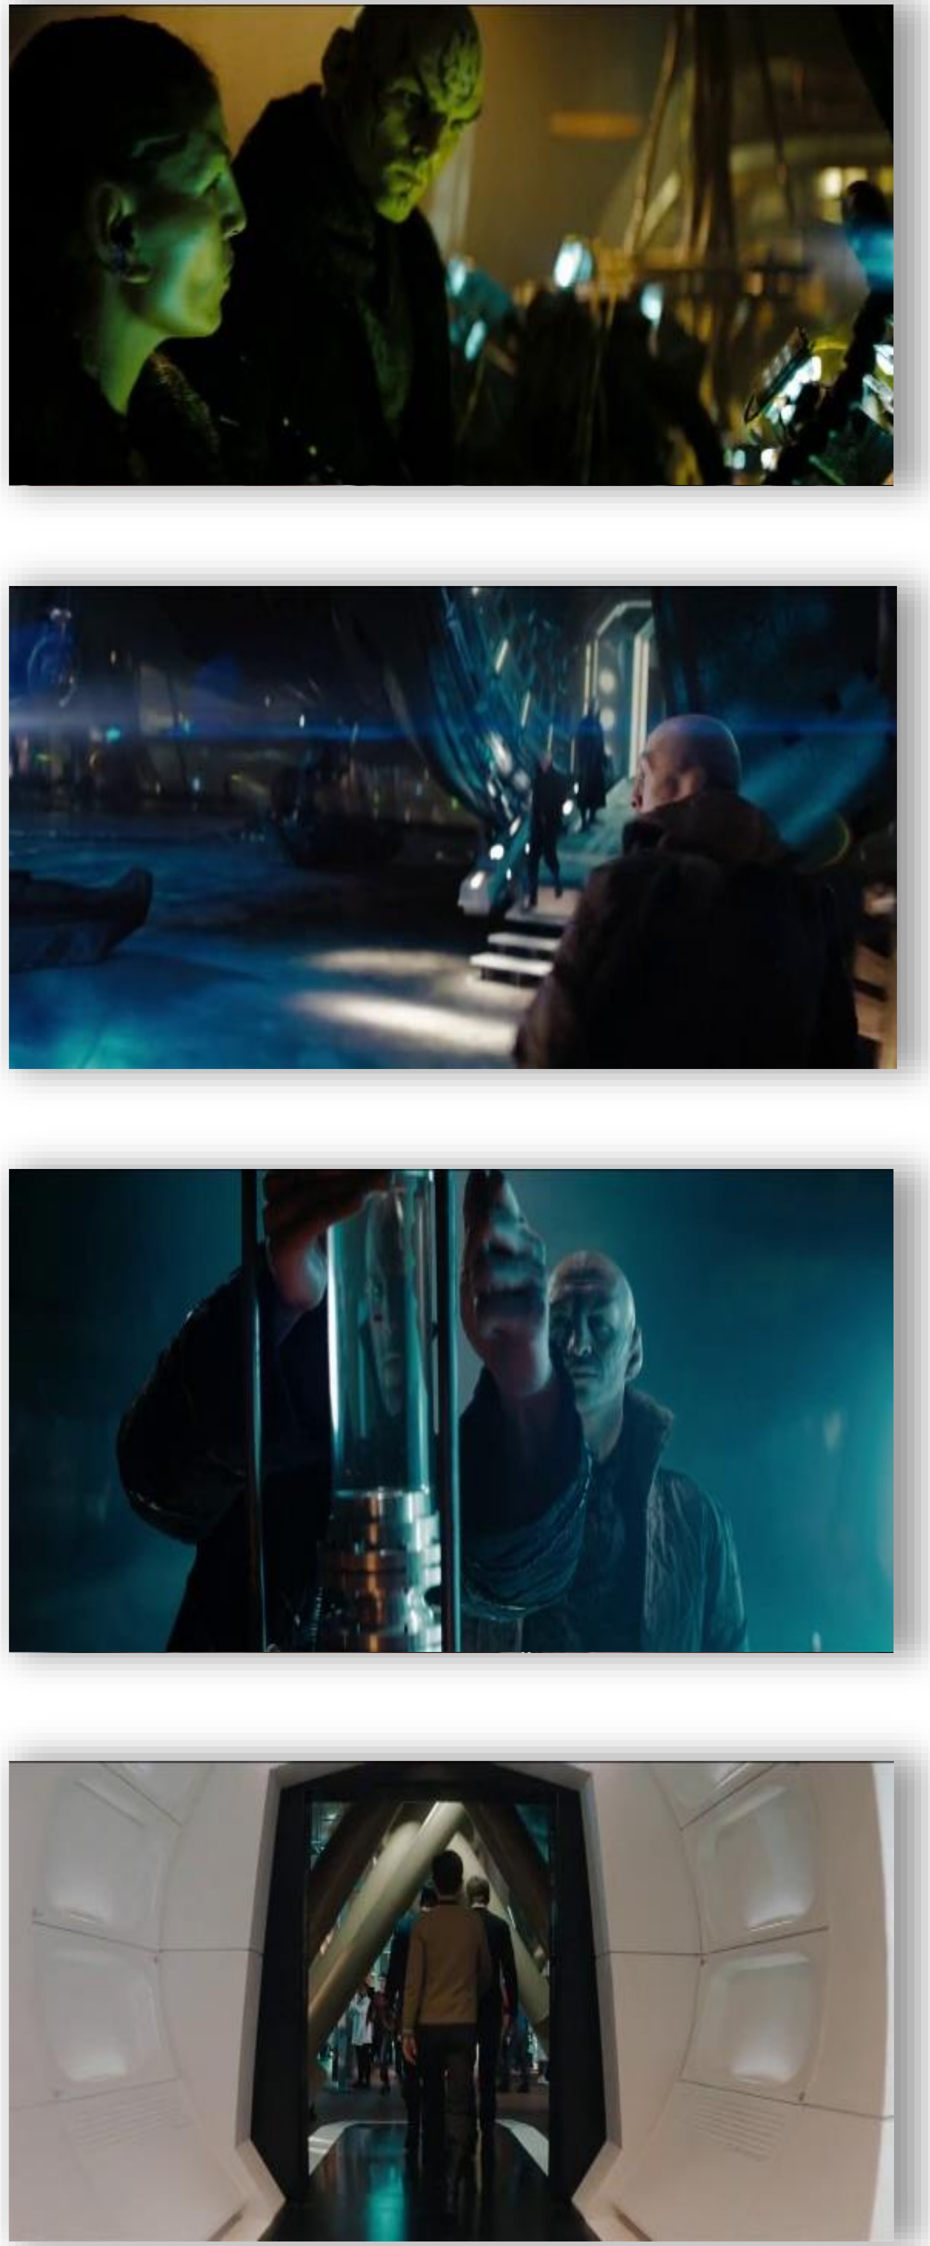

Pike promotes Spock to captain and puts him in charge of the Enterprise. He also commissions Kirk, naming him first officer, much to Spock's chagrin. Pike outlines his plan to do two things at once: from the shuttle en route to the Narada he will drop Kirk, Sulu and chief engineer Olsen into an orbital skydive. They will land on Narada's drill platform, which is deployed into the Vulcan atmosphere and is drilling a massive shaft to the core of Vulcan, causing the seismic disturbances that prompted the original distress signal. The drilling beam's signal also blocks any communication with the planet, as well as transporter beams. They will disable the drilling beam and then contact Starfleet to inform them of the incident. If all else fails, they are to fall back to the primary fleet at the Laurentian system. If Pike doesn't come back, they will also need to rescue him.

High: system | s.o.s | rescue mission | communication blockage

Medium: space shuttle | primary fleet | transporter beams | drilling platform

Low: xxx | xxx | xxx | xxx | corridor | xxx

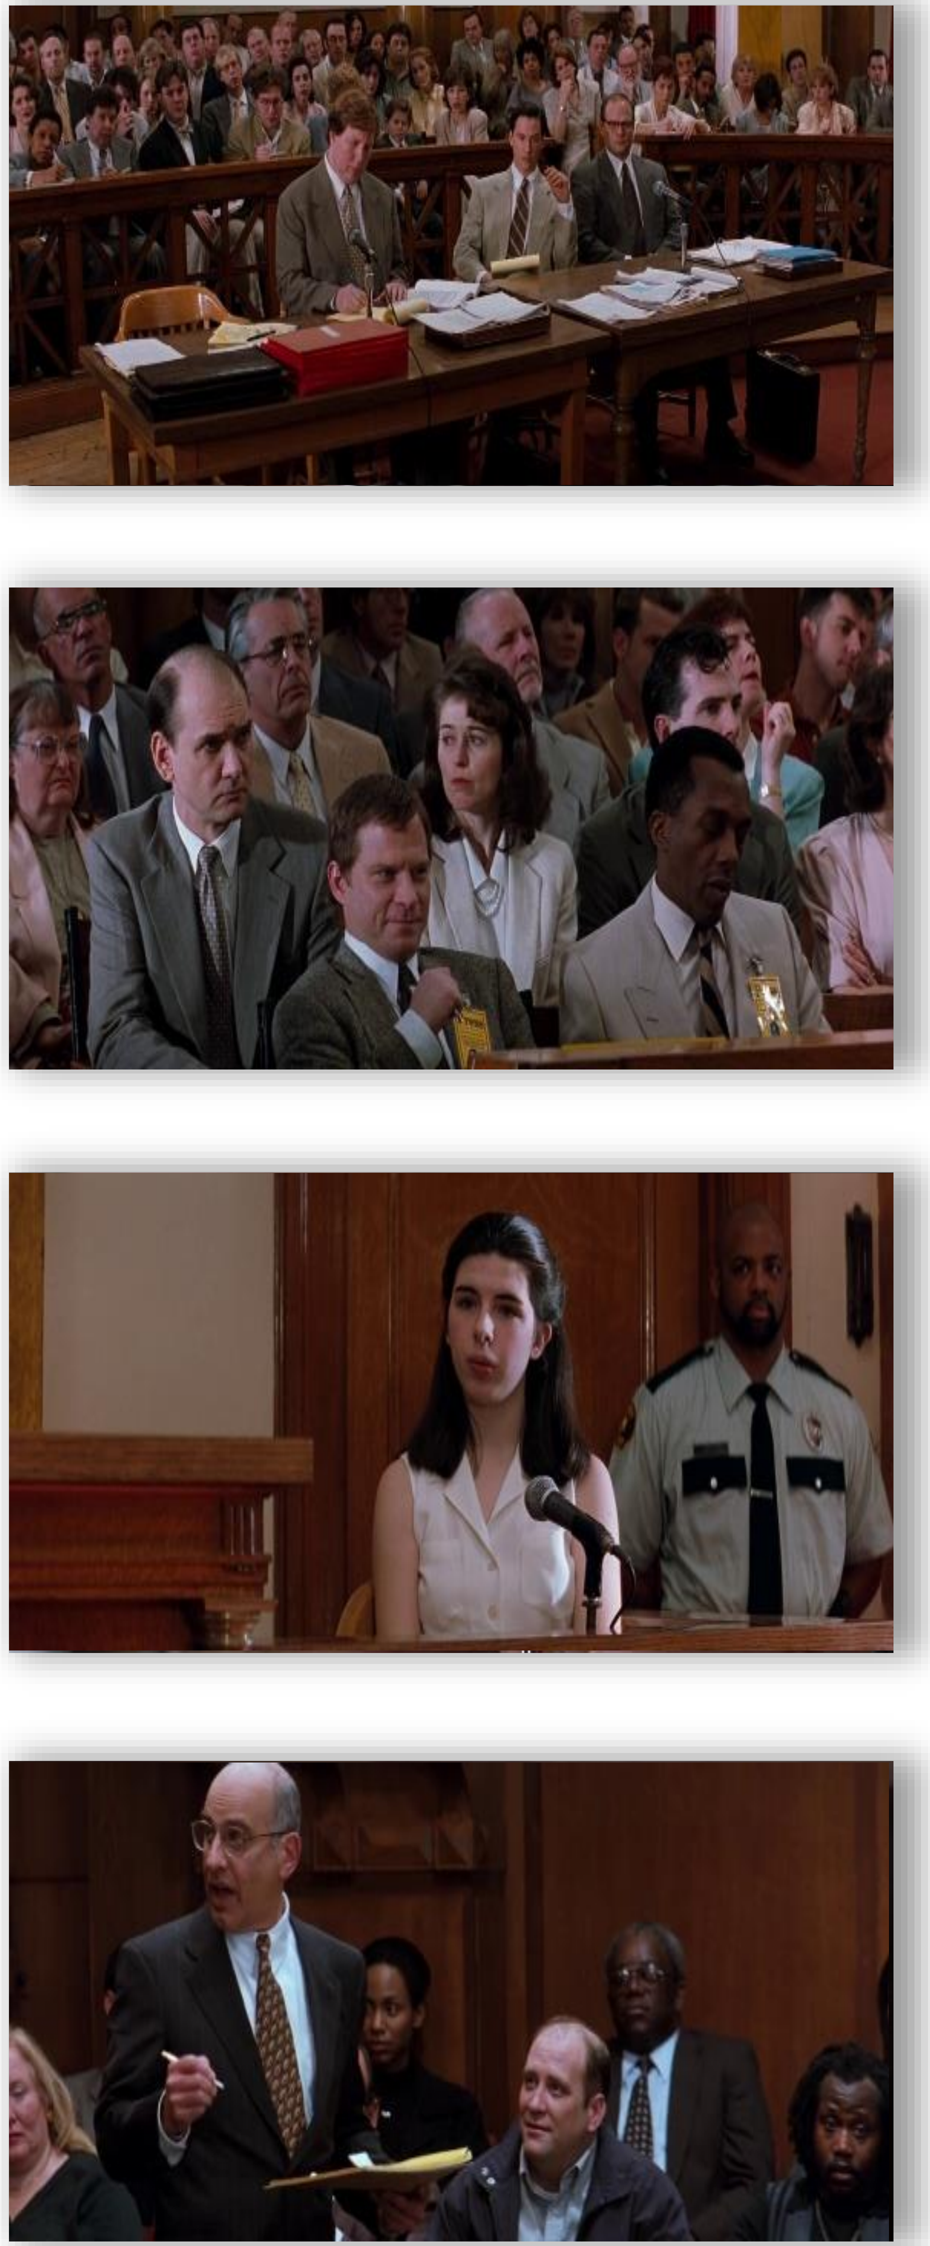

Kevin Lomax (Keanu Reeves) is a successful defense attorney in Gainesville, Florida. After successfully defending a high school teacher, Gettys, who is accused of molesting a young girl named Barbara (Heather Matarazzo). He is celebrating with his wife Mary Ann (Charlize Theron) when he is approached by a representative for a New York law firm, Leamon Heath (Ruben Santiago-Hudson). The Lomaxes go to New York, and Kevin proves his expertise while picking a jury. A sharply-dressed John Milton (Al Pacino) watches him from afar. The next day, Kevin receives word that Gettys has been acquitted. More so, the jury only deliberated for 38 minutes before bringing in the verdict.

| | |
|---|---|
| High | attorney \| high school teacher \| molesting \| defending \| girl \| jury \| verdict \| court \| deliberation |
| Medium | acquitted \| crowd \| professional knowledge \| wife \| celebrating \| representative |
| Low | paper \| clothing \| microphone \| shirt \| room |
